# Supplementary material for: Motivations, Challenges, Best Practices, and Benefits for Bots and Conversational Agents in Software Engineering: A Multivocal Literature Review
Source: arXiv:2409.11864 source file (2025-03-17)
Supplement: Supplementary file 1 [file appendix.tex]

\clearpage
\appendix

\section{Online Appendix — Supplementary Material for Methodology}
\setcounter{figure}{0} 
\setcounter{table}{0} 

\begin{figure}[H]
    \centering
    \includegraphics[width=\linewidth]{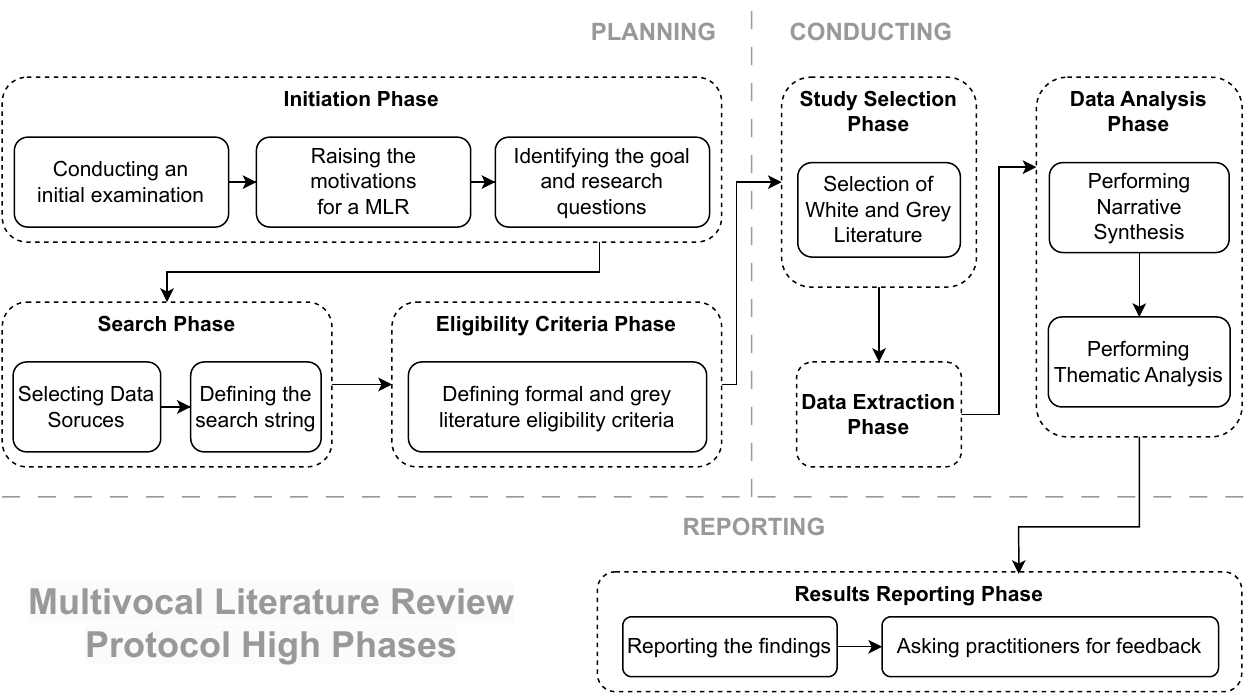}
    \caption{Overview of the methods used for the study.}
    \label{fig:methodology}
\end{figure}

\begin{figure}[H]
    \centering
    \includegraphics[width=\linewidth]{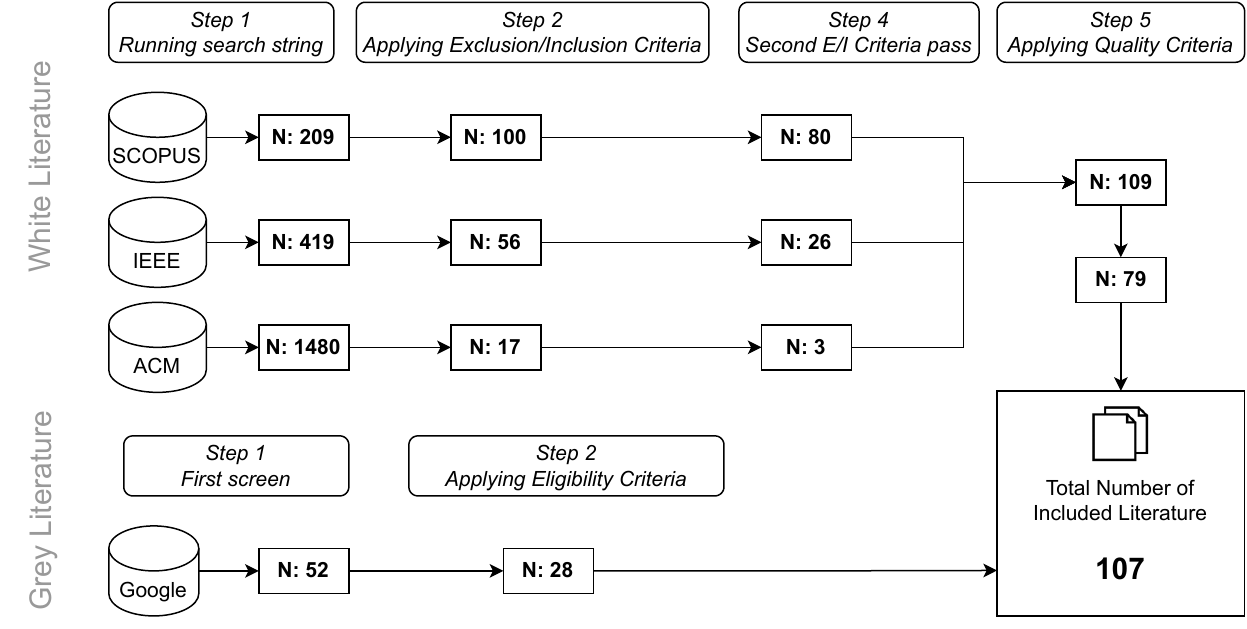}
    \caption{MLR studies selection process.}
    \label{fig:study_selection}
\end{figure}

\begin{table}[H]
    \centering
    \caption{Eligibility Criteria for Grey Literature~\cite{garousi2019_mlr_guidelines}}
    
    \rowcolors{1}{graytable}{white}
    \resizebox{\linewidth}{!}{
    \begin{tabular}{p{0.025\linewidth} p{0.15\linewidth} p{0.825\linewidth}}
        \toprule
        \rowcolor{black}
        \textbf{\textcolor{white}{\#}} & \textbf{\textcolor{white}{Category}} & \textbf{\textcolor{white}{Questions}}\\
        \bottomrule
        1 & Authority of the producer & 
        \begin{itemize}[
            nosep, left=0pt,
            before={\begin{minipage}[t]{\hsize}},
            after ={\end{minipage}} 
            ]  
            \item Is the publishing organization reputable? E.g., the Software Engineering Institute (SEI)
            \item Is an individual author associated with a reputable organization?
            \item Has the author published other work in the field?
            \item Does the author have expertise in the area? (e.g. job title principal software engineer) 
        \end{itemize}
        \\
        2 & Methodology & 
        \begin{itemize}[
            nosep, left=0pt,
            before={\begin{minipage}[t]{\hsize}},
            after ={\end{minipage}} 
            ]  
            \item Does the source have a clearly stated aim?
            \item Does the source have a stated methodology?
            \item Is the source supported by authoritative, contemporary references?
            \item Are any limits clearly stated?
            \item Does the work cover a specific question?
            \item Does the work refer to a particular population or case? 
        \end{itemize}
        \\
        3 & Objectivity &
        \begin{itemize}[
            nosep, left=0pt,
            before={\begin{minipage}[t]{\hsize}},
            after ={\end{minipage}} 
            ]  
            \item Does the work seem to be balanced in presentation?
            \item Is the statement in the sources as objective as possible? Or, is the statement a subjective opinion?
            \item Is there vested interest? E.g., a tool comparison by authors that are working for particular tool vendor
            \item Are the conclusions supported by the data? 
        \end{itemize}
        \\
        4 & Date &
        \begin{itemize}[
            nosep, left=0pt,
            before={\begin{minipage}[t]{\hsize}},
            after ={\end{minipage}} 
            ]  
            \item Does the item have a clearly stated date? 
        \end{itemize}
        \\
        5 & Related Sources &
        \begin{itemize}[
            nosep, left=0pt,
            before={\begin{minipage}[t]{\hsize}},
            after ={\end{minipage}} 
            ]  
            \item Have key related GL or formal sources been linked to / discussed? 
        \end{itemize}
        \\
        6 & Novelty &
        \begin{itemize}[
            nosep, left=0pt,
            before={\begin{minipage}[t]{\hsize}},
            after ={\end{minipage}} 
            ]  
            \item Does it enrich or add something unique to the research?
            \item Does it strengthen or refute a current position? 
        \end{itemize}
        \\
        7 & Outlet type &
        \begin{itemize}[
            nosep, left=0pt,
            before={\begin{minipage}[t]{\hsize}},
            after ={\end{minipage}} 
            ]  
            \item 1st tier GL (measure = 1): High outlet control/ High credibility: Books, magazines, theses, government reports, white papers
            \item 2nd tier GL (measure = 0.5): Moderate outlet control/ Moderate credibility: Annual reports, news articles, presentations, videos, Q/A sites (such as StackOverflow), Wiki articles
            \item 3rd tier GL (measure = 0): Low outlet control/ Low credibility: Blogs, emails, tweets 
        \end{itemize}
        \\
        \bottomrule
    \end{tabular}
    }
    
    \label{table:eligibility_criteria_grey}
\end{table}

\begin{figure}[H]
    \centering
    \includegraphics[width=0.75\linewidth]{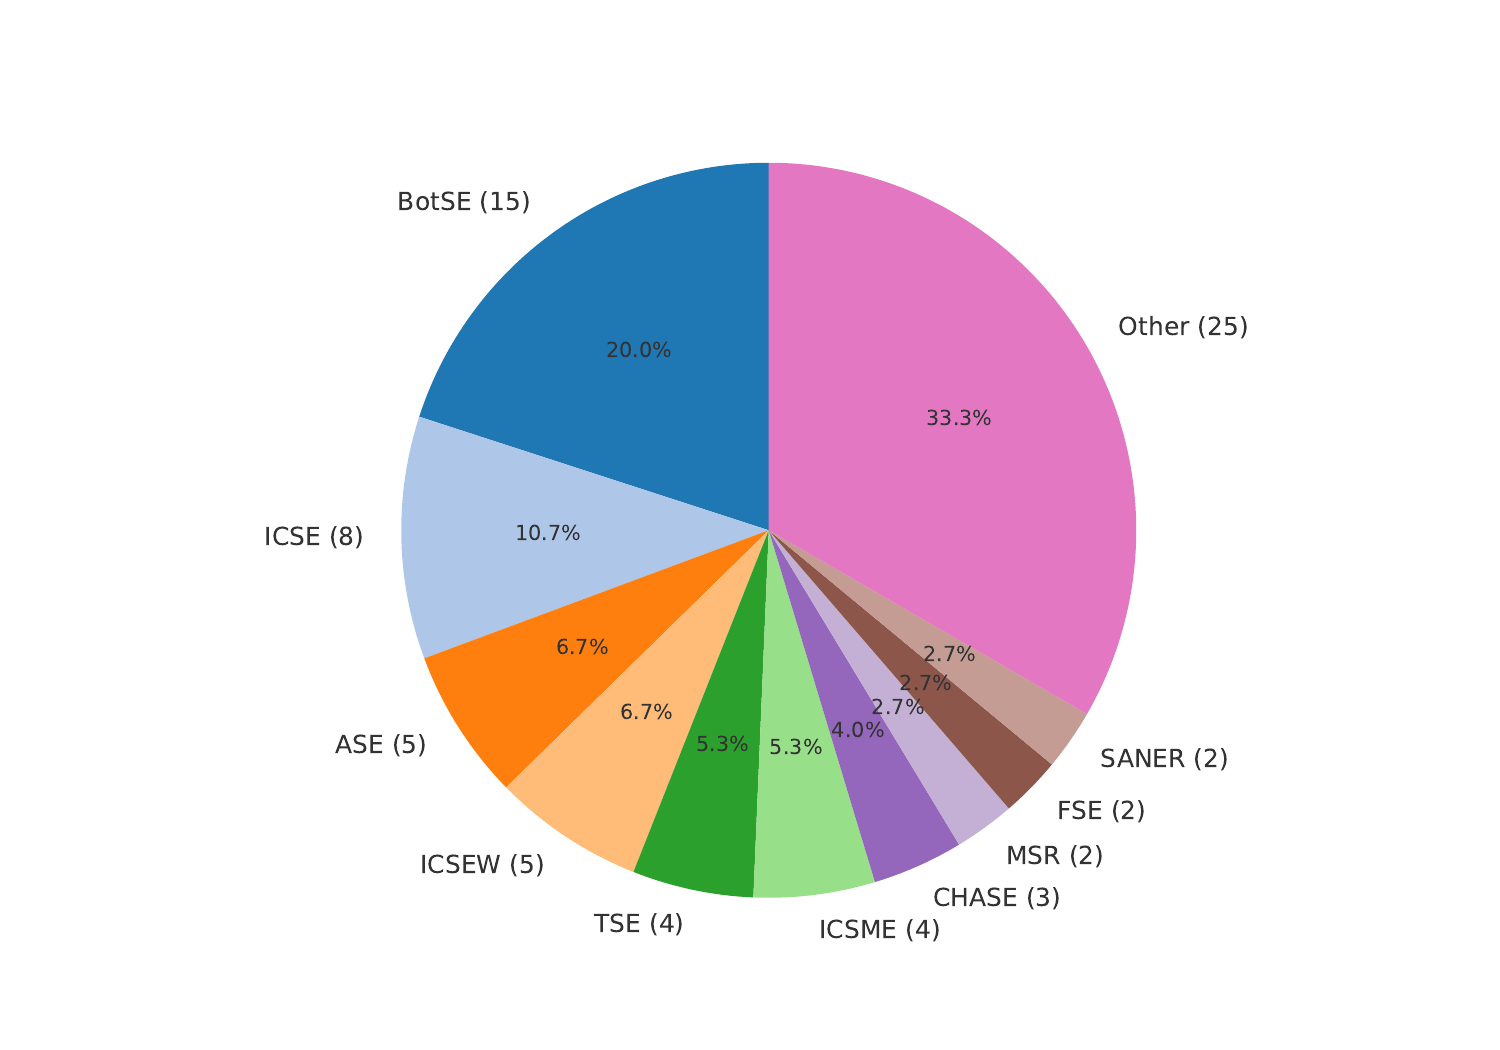}
    \caption{Selected formal literature's venues.}
    \label{fig:venues}
\end{figure}

%%%%%%%%%%%%%%%%%
%%%%%%%%%%%%%%%%%
%%%%%%%%%%%%%%%%%
\section{Online Appendix — Supplementary Material for REsults}
\setcounter{figure}{0} 
\setcounter{table}{0} 

\begin{figure}[H]
    \centering
    \includegraphics[width=1\linewidth]{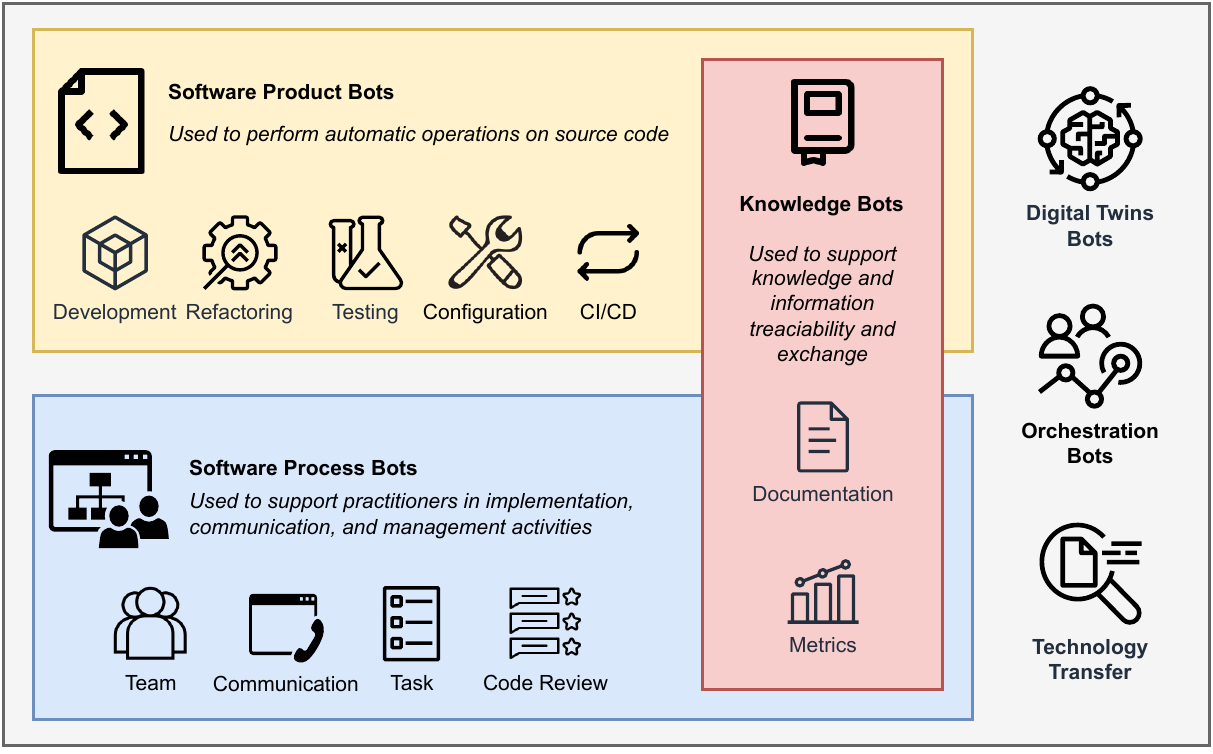}
    \caption{Motivation for adopting bots and CAs.}
    \label{fig:motivations}
\end{figure}

\begin{table}[H]
    \centering
    \caption{Identified Best Practices for \textbf{Bots Development and Design}.}
    
    \rowcolors{1}{graytable}{white}
    \resizebox{\linewidth}{!}{
    \begin{tabular}{p{0.025\linewidth} p{0.7\linewidth} p{0.275\linewidth}}
        \toprule
        \rowcolor{black}
        \textbf{\textcolor{white}{\#}} & \textbf{\textcolor{white}{Best Practice}} & \textbf{\textcolor{white}{References}}
        \\
        \bottomrule
        1 
        &
        \textit{Follow a modular architecture}
        &
        \citeA{zamanirad2017programming,lee_2019_accelerating_bots_development,srivastava_2019_architecture_applications_with_conversational_components}\citeB{understanding_CA_architecture}
        \\
        2 
        &
        \textit{Make bots adaptive and able to learn over time using AI}
        &
        \citeB{storey2020_botse,bots_challenges_for_development,bots_challenges_for_development_2}
        \\
        3
        &
        \textit{Adopt a specific lifecycle process for bots}
        &
        \citeB{implement_bot_12_steps,10_steps_for_chatbot_strategy,8_best_practices_for_bot_development}
        \\
        4 
        &
        \textit{Carefully select the correct framework based on bot requirements}
        &
        \citeB{10_best_chatbot_framework,top_framework_part_1,probot,8_chatbot_environments,abdellatif2021comparison}
        \\
        5 
        &
        \textit{Adopt Domain Specific Language Models to develop bots}
        &
        \citeA{ouaddi2024architecture,almonte2021automating}
        \\
        6
        &
        textit{Make the bot able to save and use contextual information using RAG and Vector DBs}
        &
        \citeA{arteaga2024support,de2023meet}\citeB{new_grey_3}
        \\
        7
        &
        \textit{Conduct Wizard of the Oz studies to create datasets for NL modules}
        &
        \citeA{robe2022pairProgramming_dataset}\citeB{new_grey_4}
        \\
        \bottomrule
    \end{tabular}
    }
    
    \label{table:best_practices_developmnent}
\end{table}

\begin{table}[H]
    \centering
    \caption{Frameworks for bot development.}
    
    \rowcolors{1}{graytable}{white}
    \resizebox{\linewidth}{!}{
    \begin{tabular}{p{0.15\linewidth} p{0.175\linewidth} p{0.2\linewidth} p{0.475\linewidth}}
        \toprule
        \rowcolor{black}
        \textbf{\textcolor{white}{Framework}} & \textbf{\textcolor{white}{Technology}} & \textbf{\textcolor{white}{Supported Channels}} & \textbf{\textcolor{white}{Strengths}}
        \\
        \bottomrule
        Azure Bot & 
        C\#, Java, JavaScript, and Python &
        Slack, Facebook, Website, Cortana, Skype, Teams, Telegram, \dots &
        Azure Bot Framework is a framework supported and developed by Microsoft based on the idea of creating a single bot capable of working on most communication platforms (e.g., Teams and Telegram). Moreover, such a framework can be used with a vast plethora of programming languages and integrated inside Microsoft's Azure cloud infrastructure.
        \\
        Rasa &
        Python &
        Slack, Facebook, and Telegram &
        Rasa is open-source and integrates inside it a tool to train the NLP and NLU model for chatbots. Such a tool is easy to use and with excellent performance in terms of training. Moreover, it is possible to use Rasa only for the machine learning side, avoiding the conversational part altogether.
        \\
        Dialogflow &
        Node.js &
        Slack, Facebook, Alexa, Cortana, Skype, Telegram, and Viber &
        Dialogflow is a framework developed by Google that allows developers to create bots programmatically and visually. Moreover, it allows using pre-trained NLP and NLU models, greatly simplifying the steps related to constructing artificial intelligence models.
        \\
        IBM Watson &
        Java and C++ &
        Slack and Facebook &
        IBM Watson is a framework largely used with a consequent large amount of documentation available, leading to a low barrier to entry. Moreover, it provides a visual tool for interaction workflow implementation, as well as various integrations with other platforms.
        \\
        Botpress &
        JavaScript &
        Facebbok, Website, and Telegram &
        Botpress is an open-source framework that integrates most of the necessary tools for bot deployment—e.g., NLP modules, visual editor, and deployment servers. Furthermore, it eases the development allowing developers to work and test the bot on their local machine and quickly deploy it on the server.
        \\
        Probot &
        Node.js &
        GitHub &
        Probot is an open-source framework designed to help develop automation inside the GitHub collaboration platform. Probot is easy to use and well documented, besides being the most used tool for GitHub bot development.
        \\
        \bottomrule
    \end{tabular}
    }
    
    \label{table:framework_for_bot_development}
\end{table}

\begin{table}[H]
    \centering
    \caption{Identified Best Practices for \textbf{Bots Interaction and Adoption}.}
    
    \rowcolors{1}{graytable}{white}
    \resizebox{\linewidth}{!}{
    \begin{tabular}{p{0.025\linewidth} p{0.55\linewidth} p{0.425\linewidth}}
        \toprule
        \rowcolor{black}
        \textbf{\textcolor{white}{\#}} & \textbf{\textcolor{white}{Best Practice}} & \textbf{\textcolor{white}{References}}
        \\
        \bottomrule
        1
        &
        \textit{Integrate bots actions without interrupting developer workflow}
        &
        \citeA{monperrus_2019_automated_bug_fixes,erlenhov_2020_bot_characteristics_and_challenges_from_practitioners,wessel_2021_challenges_interacting_with_bot_on_OSS,wessel2022bots_orchestratore,ribeiro2022together}\citeB{storey2020_botse,implement_bot_12_steps,10_steps_for_chatbot_strategy,8_best_practices_for_bot_development}
        \\
        2
        &
        \textit{Allow developers to edit bot configuration easily}
        &
        \citeA{van_2019_programming_repair_bots,alizadeh_2019_refbot_software_refactoring_bot,erlenhov_2020_bot_characteristics_and_challenges_from_practitioners,he2023automating,wang2023optimizingEliteDev}
        \\
        3
        &
        \textit{Provide bots with personality}
        &
        \citeA{labeuf_2017_software_bots,monperrus_2019_automated_bug_fixes,robe2022designing}\citeB{implement_bot_12_steps,10_steps_for_chatbot_strategy,8_best_practices_for_bot_development}
        \\
        4
        &
        \textit{Design a Smooth and frictionless interaction}
        &
        \citeA{labeuf_2017_software_bots,brown_2019_bots_for_effective_recommendations,melo_2020_what_do_devs_expect_from_CAs,wang2023optimizingEliteDev,robe2022designing,arteaga2024support}\citeB{storey2020_botse,implement_bot_12_steps,10_steps_for_chatbot_strategy,8_best_practices_for_bot_development}
        \\
        5
        &
        \textit{Enforce transparency in bot actions and outputs}
        &
        \citeA{labeuf_2017_software_bots,monperrus_2019_automated_bug_fixes,he2023automating,wang2023optimizingEliteDev}\citeB{storey2020_botse}
        \\
        6
        &
        \textit{Integrating concepts from behavioral science in interaction flow}
        &
        \citeA{brown_2020_recommendation_for_bot_architectures,robe2022designing}
        \\
        7
        &
        \textit{Provide users with a high level of control over bot}
        &
        \citeA{brown_2019_bots_for_effective_recommendations,alizadeh_2019_refbot_software_refactoring_bot,erlenhov_2020_bot_characteristics_and_challenges_from_practitioners,wyrich_2020_acceptance_of_refactoring_bots,melo_2020_what_do_devs_expect_from_CAs,wang2023optimizingEliteDev}\citeB{storey2020_botse}
        \\
        8 
        &
        \textit{Create a reliable test infrastructure}
        &
        \citeA{erlenhov_2020_bot_characteristics_and_challenges_from_practitioners}\citeB{bots_challenges_for_development_2}
        \\
        9       
        &
        \textit{Implement a system to evaluate bot choices}
        &
        \citeA{kumar_2019_sankie,hu2023bot,wang2023optimizingEliteDev}\citeB{storey2020_botse,understanding_CA_architecture}
        \\
        10       
        &
        \textit{Adapt the bots to the privacy policies of organizations}
        &
        \citeB{new_grey_4}
        \\
        \bottomrule
    \end{tabular}
    }
    
    \label{table:best_practices_interaction}
\end{table}

\begin{table}[H]
    \centering
    \caption{Benefits of bots usage for software engineering.}
    
    \rowcolors{1}{graytable}{white}
    \resizebox{\linewidth}{!}{
    \begin{tabular}{p{0.025\linewidth} p{0.65\linewidth} p{0.325\linewidth}}
        \toprule
        \rowcolor{black}
        \textbf{\textcolor{white}{\#}} & \textbf{\textcolor{white}{Benefit}} & \textbf{\textcolor{white}{References}}\\
        \bottomrule
        1 
        &
        Bots can increase team productivity by incentivizing developers to do a task that, without bot support, would be tedious and/or boring.
        &
        \citeA{okanovi_2020_chatbot_to_support_load_testing,gilson_2020_recording_design_decision_on_the_fly}\citeB{bots_agile,5_reasons_for_codebots,microsoft_azure_to_DevSecOps}
        \\
        2 
        &
        Bots can help developers complete tasks related to meaningful goals for projects and processes. \emph{(Productivity - Effectiveness)}
        &
        \citeA{storey_2016_bot_uses_taxonomy,labeuf_2017_software_bots,gilson_2019_NLP_and_collaborativeSE,wessel_2020_code_review_bot_OSS,gilson_2020_recording_design_decision_on_the_fly,basu_2021_bot_for_distribution_of_service_requests,wang2023optimizingEliteDev,ribeiro2022together}\citeB{bots_and_AI_in_project_management,bots_and_AI_in_project_management_2}
        \\
        3 
        &
        Bots can help developers complete tasks more quickly. \emph{(Productivity - Efficiency)}
        &
        \citeA{storey_2016_bot_uses_taxonomy,carr2016automatic,tian2017APIbot,wyrich_2019_bot_for_code_refactoring,gilson_2019_NLP_and_collaborativeSE,wessel_2020_code_review_bot_OSS,dominic_2020_bot_for_SE_newcomers,okanovi_2020_chatbot_to_support_load_testing,gilson_2020_recording_design_decision_on_the_fly,wyrich_2020_acceptance_of_refactoring_bots,zhang2024automatic,scoccia2023exploring,wang2023optimizingEliteDev,wessel2022qualityBotCodeReview,ribeiro2022together}\citeB{bots_agile,5_reasons_for_codebots,new_grey_1}
        \\
        4 
        &
        Bots can reduce project time by the fact bots can operate without a break (24/7).
        &
        \citeA{erlenhov_2020_bot_characteristics_and_challenges_from_practitioners}\citeB{best_bots_to_improve_your_software_development_process,5_reasons_for_codebots,bots_and_AI_in_project_management,bots_and_AI_in_project_management_2}
        \\
        5 
        &
        Bots can act upon a high volume of tasks quickly.
        &
        \citeA{erlenhov_2020_bot_characteristics_and_challenges_from_practitioners}\citeB{bots_agile,5_reasons_for_codebots,bots_and_AI_in_project_management,bots_and_AI_in_project_management_2,new_grey_1}
        \\
        \bottomrule
        6 
        &
        Bots can improve communication and collaboration activities.
        &
        \citeA{labeuf_2017_software_bots,matthies_2019_bot_and_agile_retrospectives,gilson_2019_NLP_and_collaborativeSE,kim_2020_bot_to_facilitate_group_discussion,gilson_2020_recording_design_decision_on_the_fly,wessel2022qualityBotCodeReview}\citeB{bots_agile,bots_and_AI_in_project_management,new_grey_1}
        \\
        7 
        &
        Bots can cut the risk of human error and positively impact risk management.
        &
        \citeB{bots_agile,5_reasons_for_codebots,why_bots_format_code,microsoft_azure_to_DevSecOps}
        \\
        8 
        &
        Bots can facilitate the adoption and integration in processes of new tools/technologies/methodologies.
        &
        \citeB{bots_agile,microsoft_azure_to_DevSecOps}
        \\
        9 
        &
        Bots can Support Decision Making.
        &
        \citeA{wessel2022bots_orchestratore}\citeB{new_grey_1}
        \\
        \bottomrule
        10 
        &
        Bots can improve source code maintainability and quality.
        &
        \citeA{carr2016automatic,wyrich_2019_bot_for_code_refactoring,alizadeh_2019_refbot_software_refactoring_bot,hu_2019_improving_feedback_pull_request_with_bots,erlenhov_2020_bot_characteristics_and_challenges_from_practitioners,okanovi_2020_chatbot_to_support_load_testing,carvalho_2020_C_3PR_fix_static_analysis_violations,gilson_2020_recording_design_decision_on_the_fly,wyrich_2020_acceptance_of_refactoring_bots,wessel2022qualityBotCodeReview,ribeiro2022together}\citeB{best_bots_to_improve_your_software_development_process,bots_agile,5_reasons_for_codebots,why_bots_format_code,microsoft_azure_to_DevSecOps}
        \\
        11 
        &
        Bots can help developers acquire new knowledge or consolidate knowledge already obtained.
        &
        \citeA{beschastnikh_2017_research_and_bot,labeuf_2017_software_bots,erlenhov_2020_bot_characteristics_and_challenges_from_practitioners,lin_2020_bot_framework_for_service_development_assistance,romero_2020_experiences_building_an_answer_bot,dominic_2020_bot_for_SE_newcomers,gilson_2020_recording_design_decision_on_the_fly}\citeB{best_bots_to_improve_your_software_development_process,microsoft_azure_to_DevSecOps,new_grey_1}
        \\
        \bottomrule
    \end{tabular}
    }
    
    \label{table:benefits}
\end{table}

\section{Online Appendix — Bibliography}

%%
%% The next two lines define the bibliography style to be used, and
%% the bibliography file.
\bibliographystyleA{unsrt}
\bibliographyA{bib/formal_literature}

\bibliographystyleB{unsrt}
\bibliographyB{bib/grey_literature}

\bibliographystyle{ACM-Reference-Format}
\bibliography{bib/bibliography}
